# Supplementary material for: Sliced gradient-enhanced Kriging for high-dimensional function approximation
Source: arXiv:2204.03562 source file (2024-01-04)
Supplement: Supplementary file 1 [file SISC_supp.tex]

\documentclass[review,supplement]{siamart}
\input{SISC_shared}
\externaldocument{SISC_main}
%
%
% Optional PDF information
\ifpdf
\hypersetup{
  pdftitle={Supplementary Materials: \TheTitle},
  pdfauthor={\TheAuthors}
}
\fi
\begin{document}

\maketitle

%
%
%%
%%%
%%%%
%%%%%
%%%%%%
\section{Supplements go here}
\label{supp:sec1}
%%
%%
%%
%%
%%%
%%%%
%%%%%
%%%%%%%
%%%%%%%%
%%%%%%%%%
\bibliographystyle{siamplain}
\bibliography{Ref}
\end{document}
